# Supplementary material for: Towards Building Multilingual Language Model for Medicine
Source: arXiv:2402.13963 source file (2024-06-02)
Supplement: Supplementary file 1 [file 06_Appendix.tex]

\section{Limitations}
While our work primarily focuses on constructing a multilingual medical corpus and enhancing the capabilities of LLMs in the medical domain across various languages, we encountered certain limitations. Our effort to gather a corpus encompassed as many languages as possible, yet we found that the availability of resources diminishes for less common languages. Additionally, varying copyright policies across different countries presented significant challenges in data collection for some languages. Balancing time and resource constraints against language diversity, we selected six widely used languages and demonstrated the efficacy of our approach in enhancing LLMs' performance in these languages. In future work, we plan to expand the MMedC to include an even broader range of languages.

As discussed in Section 4, we did not apply our enhancement method to models with more than 7 billion parameters. The reason being, even pretraining a 7-billion-parameter model on a 10-billion-token corpus for one epoch on eight A100 GPUs required 12 days, making it extremely expensive for larger LLMs. Furthermore, models with over 20 billion parameters were unfeasible to load on eight A100 GPUs using FSDP, even with a batch size of one per device. However, scaling up model size remains a potentially effective method for further improvement. Our method has shown promising results across different LLMs, and with the emergence of more advanced LLMs, we anticipate adapting our approach to enhance their domain knowledge in various languages.

Lastly, our model shares some general limitations common to LLM tasks, such as the issue of hallucination, which we have yet to address. Concerning the rationale metric in our benchmark, although we suggest a positive correlation with human ratings in Section 4.5, it still falls short in precisely measuring the true performance of models. There is still considerable work to be done before these models can be reliably applied in practical clinical settings.

\section{Ethics statement}
We take pride in our work's objective of enabling people worldwide to equally benefit from the advancements in AI for healthcare. This is achieved by developing medical LLMs that perform consistently well across various languages. In constructing the MMedC, we meticulously sourced data from publicly available e-books, carefully chosen websites, and open-source datasets. Since these data is public available and has been anonymized, this approach ensures that no sensitive information is exposed to the LLMs, and avoids personal privacy leakages. Nonetheless, it remains uncertain whether the LLMs have learned to discern the distinct national customs of different regions, or if their learning is influenced by regional customs prevalent in the most frequently occurring corpus materials. In the near future, we will release all the code and data, which simultaneously promotes the development of multilingual language models and medical language models.

\section{Case Study}
\label{sec:case_show}

In this study, we analyzed individual cases across various languages. We specifically compared the responses of MMedLM and Internlm, noting that MMedLM represents an advanced iteration of Internlm, augmented with domain-specific knowledge. As illustrated in Figures~\ref{fig:case1}, \ref{fig:case2}, \ref{fig:case3}, \ref{fig:case4}, \ref{fig:case5}, and \ref{fig:case6}, MMedLM consistently demonstrates superior performance in selecting the correct option, unlike Internlm. Furthermore, MMedLM frequently justifies its choices with accurate reasons. For instance, in Figure~\ref{fig:case1}, MMedLM accurately diagnoses 'eosinophilic infiltration in the renal biopsy,' subsequently applying its domain knowledge to identify these findings as indicative of toxic tubulointerstitial nephritis, leading to a precise diagnosis.

Nevertheless, we also notice an exception in Figure~\ref{fig:case5}, where the language model (LLM) correctly identifies the answer, but with an erroneous rationale. Although the model attributes apoptosis to viral infections by stating that 'viruses attack cells, causing apoptosis,' it overlooks the fact that apoptosis is, in reality, an active defense mechanism employed by the body to curb viral replication. This observation suggests that the model's selection of the correct answer could be attributed to chance rather than a genuine understanding or possession of relevant knowledge. It further underscores the importance of evaluating not only the accuracy of the model's answers but also its reasoning process. 

\section{Implement details}
\label{sec:implement_details}
In this section, we delve into the specifics of pretraining and finetuning. Throughout our experiments, which were conducted using the PyTorch framework and the Transformers library, we consistently set the random seed to 42. 
\subsection{Pretraining stage}
During the pretraining phase, our optimization objective aligns with that of the autoregressive generation task. For data processing, we segment the text from each .txt file into chunks, each comprising 2048 tokens, with an overlapping margin of 512 tokens. Throughout the training, we maintain a maximum context length of 2048 tokens. Owing to the model's extensive parameter count, which precludes fitting on a single GPU, we employ the Fully Sharded Data Parallel (FSDP) strategy to distribute the model across multiple GPU cards. Additionally, we utilize the BF16 data type and gradient checkpointing techniques to optimize memory usage. For InternLM, we establish a global batch size of 512 and a learning rate of 2e-5. In the case of BLOOM, we set the global batch size to 512 and a learning rate of 8e-6. We pretrain both models on eight A100 GPUs, adapting gradient accumulation steps to sustain such a large global batch size. We pretrain the 7B model for 20000 iterations, which takes about 20 Days.
\subsection{Finetuning stage}
To have a better evaluation of model's performance, we finetuned models on the trainset of MMedB. During the fine-tuning process, our optimization objective remained consistent with the pretraining phase, focusing on autoregressive generation. However, unlike pretraining, the loss was calculated not over the entire sentence outputted by the model, but solely on the tokens in the response part. We set the maximum sequence length to 2048, padding each batch to match the longest sequence in that batch. Similar to the pretraining setup, we utilized Fully Sharded Data Parallel (FSDP), BF16 data type, and gradient checkpointing technology. For all models, we established a global batch size of 128 and a learning rate of 1e-6. Each model was trained on four A100 GPUs for five epochs, which takes approximately 12 hours.

\subsection{Prompt Used}
\label{sec:prompt_used}
In this section, we introduce the prompts used in the experiments.
\subsubsection{Zero-shot prompt}
For models such as GPT-3.5 and GPT-4, we employ specific instructions to steer the model's response to questions. To prompt the model for a straightforward correct answer, we use the following directive: 
\begin{mdframed}[backgroundcolor=gray!20]
You're a {lang} doctor, make a choice based on the question and options. You need to answer the letter of the option instead of answering the entire option or anything else. Options may not be unique
\end{mdframed}
Conversely, when we aim for the model to provide not just the correct answer but also its corresponding rationale, we utilize a different instruction: 
\begin{mdframed}[backgroundcolor=gray!20]
You're a {lang} doctor, make a choice based on the question and options in {lang}. You should solve this step-bystep. You must first give the reason in {lang} for your choice end with '[End]'. Then you must give the answer's letter directly again. The temlpate is like 'Reason:... [End] Answer: A,B'
\end{mdframed}
\subsubsection{Finetune prompt}
Similar to the prompting technique employed in GPT models, we utilize two distinct types of prompts in our approach. For eliciting a direct, straightforward answer, we apply the following prompt: 
\begin{mdframed}[backgroundcolor=gray!20]
You're a {lang} doctor, kindly address the medical queries according to the patient's account. Answer with the best option directly.
\end{mdframed}
In contrast, to obtain an answer accompanied by its corresponding rationale, we use a more detailed prompt: 
\begin{mdframed}[backgroundcolor=gray!20]
You're a {lang} doctor, kindly address the medical queries according to the patient's account in {lang}. Let’s solve this step-by-step.  You should first give the reason in {lang} for your choice. Then you should give the right answer index of the question.
\end{mdframed}
It is important to note that during finetuning, we employed both of the aforementioned instructions. This implies that for each sample, the model underwent optimization twice in each epoch, with different instructions and corresponding outputs. During evaluation, the first instruction was used to determine the model's accuracy, owing to its significant convenience in metric calculation. Conversely, the second instruction was utilized to generate rationales and to assess their similarity with the reference material.

\subsubsection{Ranking Prompt}
We used the following instruction for rating the rationales with GPT4.
\begin{mdframed}[backgroundcolor=gray!20]
Please act as an impartial judge and evaluate the quality of the responses provided by six
AI assistants to the user question displayed below. You should choose the assistant that
follows the user’s instructions and answers the user’s question better. Your evaluation
should consider factors such as the helpfulness, relevance, accuracy, depth, creativity,
and level of detail of their responses. Begin your evaluation by comparing the six
responses. Avoid any position biases and ensure that the
order in which the responses were presented does not influence your decision. Do not allow
the length of the responses to influence your evaluation. Do not favor certain names of
the assistants. Be as objective as possible. Your output is the ordering of these six models by from high to low. Output your
final verdict from high to low by strictly following this format: Model A, Model B, Model C, Model D, Model E, Model F.
\end{mdframed}

\subsection{Human Evaluation}
We provide a detailed introduction to the process of manual evaluation. We employed five medical students from China for this task, including one Ph.D. student, three Master's students, and one undergraduate student. The evaluation criteria are as follows:
\begin{itemize}
    \item Accuracy: The model's ability to correctly select the answer.
    \item Reasoning Ability: The model's capacity to demonstrate logical reasoning in making its selection. The model should go beyond merely repeating the question or options, supporting its choice with reasonable reasoning.
    \item Integration of Internal Knowledge: The model needs to effectively blend and utilize its internal knowledge base, providing relevant and persuasive factual evidence to support its answer.
\end{itemize}

For each sample, annotators were required to rank the models based on these three criteria. We compensated 3 CNY(0.42 USD) for each case.

\section{Detailed results}
\subsection{Accuracy on ablation study}
\pengcheng{Need to report language-wise accuracy during ablation study.}

\subsection{Different metrics on rationale evaluation}
We conducted an in-depth analysis of the scores assigned to the rationales generated by various models, utilizing a range of evaluation metrics. Figure~\ref{tab:BLEU} illustrates the performance of each model as measured by the N-gram BLEU metric. Meanwhile, Figure~\ref{tab:ROUGE} presents the scores achieved by these models under the N-gram Rouge metric.
\begin{table}[!ht]
    \centering
    \caption{Scores of n-gram BLEU}
    \label{tab:BLEU}
    \begin{tabular}{cc|cccccc|c}
    \toprule
        model & metric & EN & ZH & JA & FR & RU & ES & AVG  \\
    \toprule
        InternLM(baseline) & BLEU-1 & 46.53\% & 48.24\% & 44.89\% & 41.80\% & 27.87\% & 43.42\% & 42.12\%  \\ 
        BLOOM & BLEU-1 & 45.94\% & 48.37\% & 44.71\% & 44.47\% & 29.95\% & 45.91\% & 43.22\%  \\ 
        Llama\ 2 & BLEU-1 & 46.87\% & 46.62\% & 48.53\% & 44.43\% & 33.05\% & 45.96\% & 44.24\%  \\ 
        MedAlpaca & BLEU-1 & 47.33\% & 45.72\% & 45.35\% & 43.78\% & 32.80\% & 45.99\% & 43.49\%  \\ 
        ChatDoctor & BLEU-1 & 47.22\% & 44.66\% & 38.87\% & 44.64\% & 32.19\% & 45.68\% & 42.21\%  \\ 
        PMC\_LLaMA & BLEU-1 & 47.33\% & 45.87\% & 44.52\% & 43.80\% & 31.14\% & 46.30\% & 43.16\%  \\ 
        medInternLM-EN & BLEU-1 & 46.96\% & 48.25\% & 45.70\% & 41.61\% & 26.27\% & 43.93\% & 42.12\%  \\ 
        medInternLM-OCR & BLEU-1 & 47.46\% & 49.24\% & 47.61\% & 44.01\% & 32.42\% & 46.00\% & 44.46\%  \\ 
        medInternLM & BLEU-1 & 47.37\% & 48.68\% & 48.95\% & 45.39\% & 33.24\% & 46.68\% & 45.05\%  \\ 
    \midrule
        InternLM(baseline) & BLEU-2 & 18.76\% & 18.79\% & 18.55\% & 15.89\% & 7.44\% & 15.89\% & 15.89\%  \\ 
        BLOOM & BLEU-2 & 17.93\% & 18.70\% & 17.89\% & 18.29\% & 8.58\% & 17.69\% & 16.51\%  \\ 
        Llama\ 2 & BLEU-2 & 18.53\% & 16.98\% & 20.42\% & 17.72\% & 9.40\% & 17.31\% & 16.73\%  \\ 
        MedAlpaca & BLEU-2 & 19.30\% & 16.41\% & 18.48\% & 17.82\% & 9.90\% & 17.91\% & 16.64\%  \\ 
        ChatDoctor & BLEU-2 & 19.50\% & 16.29\% & 15.36\% & 18.25\% & 9.76\% & 17.87\% & 16.17\%  \\ 
        PMC\_LLaMA & BLEU-2 & 20.05\% & 16.28\% & 17.67\% & 17.99\% & 9.10\% & 17.68\% & 16.46\%  \\ 
        medInternLM-EN & BLEU-2 & 19.20\% & 18.50\% & 19.13\% & 15.61\% & 6.55\% & 16.39\% & 15.90\%  \\ 
        medInternLM-OCR & BLEU-2 & 19.66\% & 19.13\% & 20.44\% & 17.89\% & 9.91\% & 18.00\% & 17.50\%  \\ 
        medInternLM & BLEU-2 & 19.39\% & 18.84\% & 21.63\% & 19.46\% & 10.13\% & 18.99\% & 18.07\%  \\ 
    \midrule
        InternLM(baseline) & BLEU-3 & 9.20\% & 9.05\% & 9.56\% & 7.56\% & 3.09\% & 7.24\% & 7.62\%  \\ 
        BLOOM & BLEU-3 & 8.39\% & 8.97\% & 8.90\% & 9.15\% & 3.66\% & 8.42\% & 7.92\%  \\ 
        Llama\ 2 & BLEU-3 & 8.89\% & 7.64\% & 10.41\% & 8.78\% & 3.63\% & 7.98\% & 7.89\%  \\ 
        MedAlpaca & BLEU-3 & 9.62\% & 7.66\% & 9.39\% & 8.98\% & 4.16\% & 8.65\% & 8.08\%  \\ 
        ChatDoctor & BLEU-3 & 9.62\% & 7.34\% & 7.74\% & 9.17\% & 4.10\% & 8.63\% & 7.77\%  \\ 
        PMC\_LLaMA & BLEU-3 & 10.14\% & 7.27\% & 8.91\% & 8.91\% & 3.88\% & 8.46\% & 7.93\%  \\ 
        medInternLM-EN & BLEU-3 & 9.42\% & 8.85\% & 10.08\% & 7.40\% & 2.58\% & 7.72\% & 7.67\%  \\ 
        medInternLM-OCR & BLEU-3 & 9.79\% & 9.09\% & 10.68\% & 8.90\% & 3.86\% & 8.71\% & 8.50\%  \\ 
        medInternLM & BLEU-3 & 9.55\% & 9.20\% & 11.84\% & 10.24\% & 4.20\% & 9.38\% & 9.07\%  \\ 
    \midrule
        InternLM(baseline) & BLEU-4 & 5.23\% & 4.82\% & 5.51\% & 3.88\% & 1.55\% & 3.90\% & 4.15\%  \\ 
        BLOOM & BLEU-4 & 4.55\% & 4.62\% & 4.87\% & 4.73\% & 1.76\% & 4.58\% & 4.18\%  \\ 
        Llama\ 2 & BLEU-4 & 4.85\% & 3.67\% & 5.94\% & 4.66\% & 1.66\% & 4.28\% & 4.17\%  \\ 
        MedAlpaca & BLEU-4 & 5.43\% & 3.88\% & 5.33\% & 4.83\% & 1.95\% & 4.89\% & 4.38\%  \\ 
        ChatDoctor & BLEU-4 & 5.47\% & 3.65\% & 4.42\% & 4.86\% & 1.96\% & 4.71\% & 4.18\%  \\ 
        PMC\_LLaMA & BLEU-4 & 5.79\% & 3.58\% & 5.04\% & 4.52\% & 1.93\% & 4.66\% & 4.25\%  \\ 
        medInternLM-EN & BLEU-4 & 5.31\% & 4.64\% & 5.87\% & 3.74\% & 1.20\% & 4.27\% & 4.17\%  \\ 
        medInternLM-OCR & BLEU-4 & 5.62\% & 4.71\% & 6.13\% & 4.73\% & 1.77\% & 4.84\% & 4.63\%  \\ 
        medInternLM & BLEU-4 & 5.42\% & 5.02\% & 7.09\% & 5.71\% & 1.88\% & 5.39\% & 5.08\%  \\ 
    \midrule
    \end{tabular}
\end{table}

\begin{table}[!ht]
    \centering
    \caption{Scores of n-gram Rouge}
    \label{tab:ROUGE}
    \begin{tabular}{cc|cccccc|c}
    \toprule
        model & metric & EN & ZH & JA & FR & RU & ES & AVG  \\
    \toprule
        InternLM(baseline) & rouge1 & 41.86\% & 48.64\% & 49.83\% & 37.95\% & 21.20\% & 38.59\% & 39.68\%  \\ 
        BLOOM & rouge1 & 40.51\% & 48.26\% & 48.61\% & 41.05\% & 21.50\% & 40.77\% & 40.12\%  \\ 
        Llama\ 2 & rouge1 & 41.39\% & 46.57\% & 51.21\% & 40.38\% & 23.24\% & 40.37\% & 40.53\%  \\ 
        MedAlpaca & rouge1 & 42.31\% & 46.49\% & 49.12\% & 40.41\% & 23.15\% & 40.57\% & 40.34\%  \\ 
        ChatDoctor & rouge1 & 41.97\% & 45.81\% & 47.95\% & 40.25\% & 23.37\% & 40.71\% & 40.01\%  \\ 
        PMC\_LLaMA & rouge1 & 42.87\% & 46.18\% & 48.44\% & 40.23\% & 22.28\% & 40.68\% & 40.12\%  \\ nm=
        medInternLM-EN & rouge1 & 42.42\% & 48.92\% & 50.22\% & 38.36\% & 19.88\% & 39.16\% & 39.83\%  \\ 
        medInternLM-OCR & rouge1 & 42.65\% & 49.91\% & 50.81\% & 40.42\% & 24.00\% & 40.43\% & 41.37\%  \\ 
        medInternLM & rouge1 & 41.98\% & 49.28\% & 52.34\% & 41.41\% & 24.67\% & 41.35\% & 41.84\%  \\
    \midrule
        InternLM(baseline) & rouge2 & 16.19\% & 19.86\% & 22.13\% & 14.67\% & 5.64\% & 14.92\% & 15.57\%  \\ 
        BLOOM & rouge2 & 15.25\% & 19.78\% & 21.22\% & 16.63\% & 6.13\% & 16.44\% & 15.91\%  \\ 
        Llama\ 2 & rouge2 & 15.75\% & 18.07\% & 22.81\% & 15.76\% & 6.33\% & 15.81\% & 15.76\%  \\ 
        MedAlpaca & rouge2 & 16.41\% & 17.63\% & 21.78\% & 16.21\% & 7.11\% & 16.49\% & 15.94\%  \\ 
        ChatDoctor & rouge2 & 16.70\% & 17.67\% & 20.65\% & 16.16\% & 7.12\% & 16.64\% & 15.82\%  \\ 
        PMC\_LLaMA & rouge2 & 17.40\% & 17.56\% & 21.00\% & 16.20\% & 6.77\% & 16.47\% & 15.90\%  \\ 
        medInternLM-EN & rouge2 & 16.58\% & 19.71\% & 22.63\% & 14.47\% & 5.23\% & 15.21\% & 15.64\%  \\ 
        medInternLM-OCR & rouge2 & 16.78\% & 20.23\% & 23.39\% & 16.25\% & 7.31\% & 16.60\% & 16.76\%  \\ 
        medInternLM & rouge2 & 16.31\% & 20.00\% & 24.50\% & 17.82\% & 7.57\% & 17.56\% & 17.29\%  \\
    \midrule
        InternLM(baseline) & rougel & 37.89\% & 33.59\% & 32.49\% & 34.37\% & 20.13\% & 34.26\% & 32.12\%  \\ 
        BLOOM & rougel & 36.53\% & 32.84\% & 32.03\% & 37.17\% & 19.90\% & 35.94\% & 32.40\%  \\ 
        Llama\ 2 & rougel & 37.05\% & 31.09\% & 32.45\% & 36.44\% & 21.73\% & 35.72\% & 32.41\%  \\ 
        MedAlpaca & rougel & 38.00\% & 31.43\% & 32.08\% & 36.57\% & 21.77\% & 36.13\% & 32.66\%  \\ 
        ChatDoctor & rougel & 37.91\% & 31.04\% & 31.62\% & 36.29\% & 22.02\% & 36.38\% & 32.54\%  \\ 
        PMC\_LLaMA & rougel & 38.77\% & 30.85\% & 31.42\% & 36.57\% & 21.13\% & 36.19\% & 32.49\%  \\ 
        medInternLM-EN & rougel & 38.20\% & 34.29\% & 33.05\% & 34.61\% & 18.78\% & 34.91\% & 32.31\%  \\ 
        medInternLM-OCR & rougel & 38.66\% & 34.62\% & 32.95\% & 36.40\% & 22.63\% & 36.46\% & 33.62\%  \\ 
        medInternLM & rougel & 37.84\% & 34.35\% & 34.51\% & 37.81\% & 23.19\% & 37.08\% & 34.13\%  \\
    \midrule
    \end{tabular}
\end{table}

\begin{table}[!ht]
    \centering
    \caption{Scores of GPT4 rating}
    \label{tab:gpt4_rating}
    \begin{tabular}{c|cccccc|c}
    \toprule
        model & EN & ZH & JA & FR & RU & ES & AVG  \\
    \toprule
        Med-InternLM & 4.12 & 4.74 & 4.44 & 4.44 & 4.22 & 4.36 & 4.39  \\
        InternLM & 3.58 & 4.04 & 3.26 & 2.74 & 2.64 & 2.8 & 3.18  \\ 
        BLOOM & 2.68 & 3.18 & 3.02 & 3.2 & 3.28 & 3.22 & 3.1  \\ 
        Llama\ 2 & 3.24 & 3.2 & 3.46 & 3.2 & 4.18 & 3.72 & 3.5  \\ 
        PMC-LLaMA & 4.3 & 3.22 & 3.06 & 3.22 & 3.26 & 3.2 & 3.38  \\ 
        GPT-3.5 & 3.08 & 2.62 & 3.76 & 4.2 & 3.42 & 3.7 & 3.46  \\ 
    \midrule
    \end{tabular}
\end{table}

\begin{table}[!ht]
    \centering
    \caption{Scores of human rating}
    \label{tab:human_rating}
    \begin{tabular}{c|cccccc|c}
    \toprule
        model & EN & ZH & JA & FR & RU & ES & AVG  \\
    \toprule
    Med-InternLM & 4.3 & 4.78 & 4.94 & 4.14 & 4.44 & 4.66 & 4.54  \\
    InternLM & 3.68 & 3.94 & 3.78 & 3.44 & 2.92 & 2.62 & 3.4  \\ 
    BLOOM & 3.2 & 3.6 & 3.16 & 3.3 & 3.34 & 3.26 & 3.31  \\ 
    Llama\ 2 & 3.14 & 3.48 & 3.52 & 3.5 & 3.68 & 3.96 & 3.55  \\ 
    PMC-LLaMA & 3.44 & 2.72 & 2.82 & 3.2 & 3.38 & 3.16 & 3.12  \\ 
    GPT-3.5 & 3.24 & 2.48 & 2.78 & 3.42 & 3.24 & 3.34 & 3.08  \\
    \midrule
    \end{tabular}
\end{table}

\subsection{Correlation between Human and Automatic Metrics}
We also analyse the correlation between human rating result and automatic metrics. 
\begin{figure}[t]
    \centering
    \includegraphics[width=\textwidth]{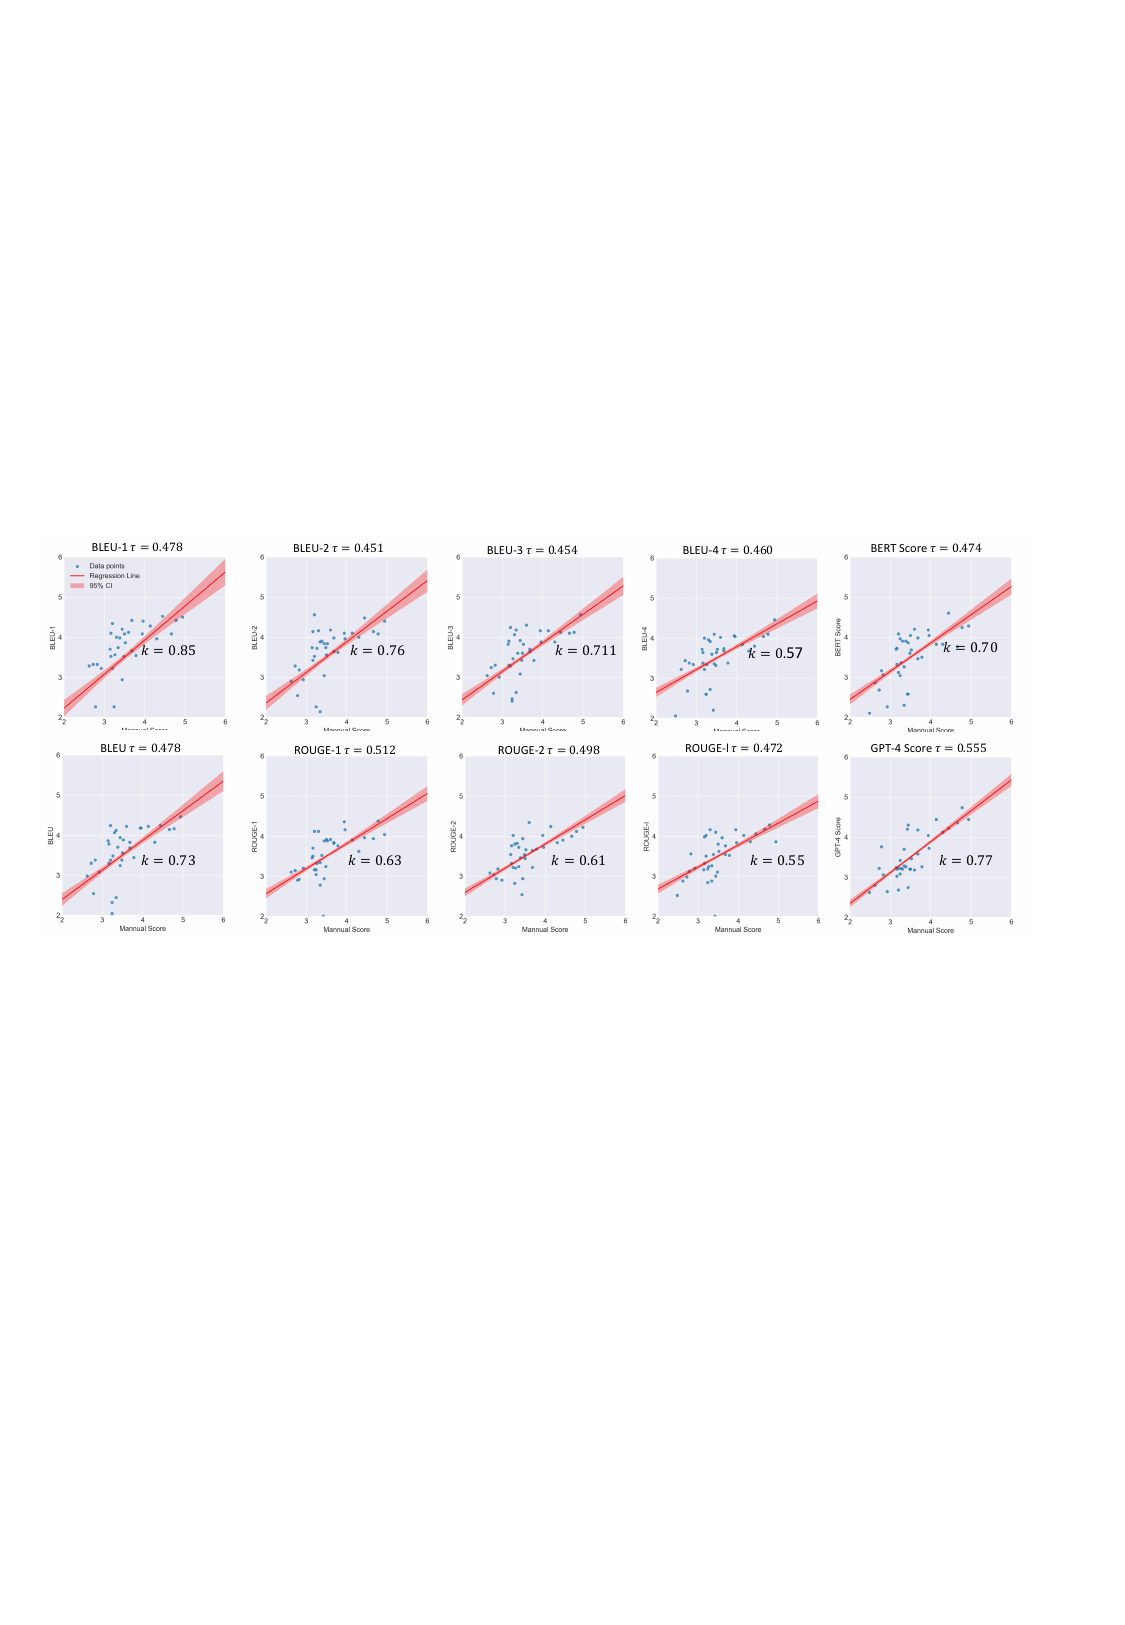}
    \vspace{-10pt}
    \caption{Correlation between human rating result and automatic metrics}
    \label{fig:correlation_analyse}
\end{figure}

\section{Websites involved}
\subsection{Websites for crawling}
\label{sec:websites_for_crawling}
Our research involved extensive data collection from various medical websites. These websites were methodically crawled to gather comprehensive data. Below is a list of the key websites included in our data collection process:
\begin{enumerate}
    \item Nikkei Medical Online - Guidelines and Protocols \url{https://medical.nikkeibp.co.jp/inc/all/dic/guideline/}
    \item Jiji Medical - Medical News and Articles \url{https://medical.jiji.com/}
    \item InnerVision - Diagnostic Imaging Insights \url{https://www.innervision.co.jp/}
    \item QLifePro - Latest Medical Research and Trends \url{https://www.qlifepro.com/}
    \item MedicalNote - Disease Index and Information \url{https://medicalnote.jp/diseases/list/name_line_a}
    \item DoctorsFile - Medication and Treatment Database \url{https://doctorsfile.jp/medication/556/}
    \item Cancer Information Japan - Comprehensive Cancer Resources \url{https://www.cancerit.jp/gann-kiji-itiran/}
    \item Japan Medical News Network - Editorials and Healthcare Discussions \url{https://www.jmnn.jp/archives/category/edit}
    \item QLife - Medicine and Drug Information \url{https://www.qlife.jp/meds/}
    \item MedlinePlus - Trusted Health Information \url{https://medlineplus.gov/}
    \item Pasteur Institute - Disease Fact Sheets \url{https://www.pasteur.fr/fr/centre-medical/fiches-maladies}
\end{enumerate}
\subsection{Websites for free ebooks}
\begin{enumerate}
    \item  A collection of French-language medical literature and historical documents \url{https://collections.nlm.nih.gov/?f%5Bdrep2.language%5D%5B%5D=French }
    \item  A portal for downloading ebooks on Traditional Chinese Medicine \url{http://www.a-hospital.com/w/%E5%88%86%E7%B1%BB:%E4%B8%AD%E5%8C%BB%E7%94%B5%E5%AD%90%E4%B9%A6%E4%B8%8B%E8%BD%BD}
    \item  Library Genesis provides free ebooks mainly in Russian covering various topics \url{https://libgen.is/search.php?req=la+diabetes&lg_topic=libgen&open=0&view=simple&res=25&phrase=1&column=def}
    \item  DoctorPDF provides access to Spanish medical books in PDF format \url{https://doctorpdf.org/libros/}
\end{enumerate}

\begin{figure}[t]
    \centering
    \includegraphics[width=\textwidth]{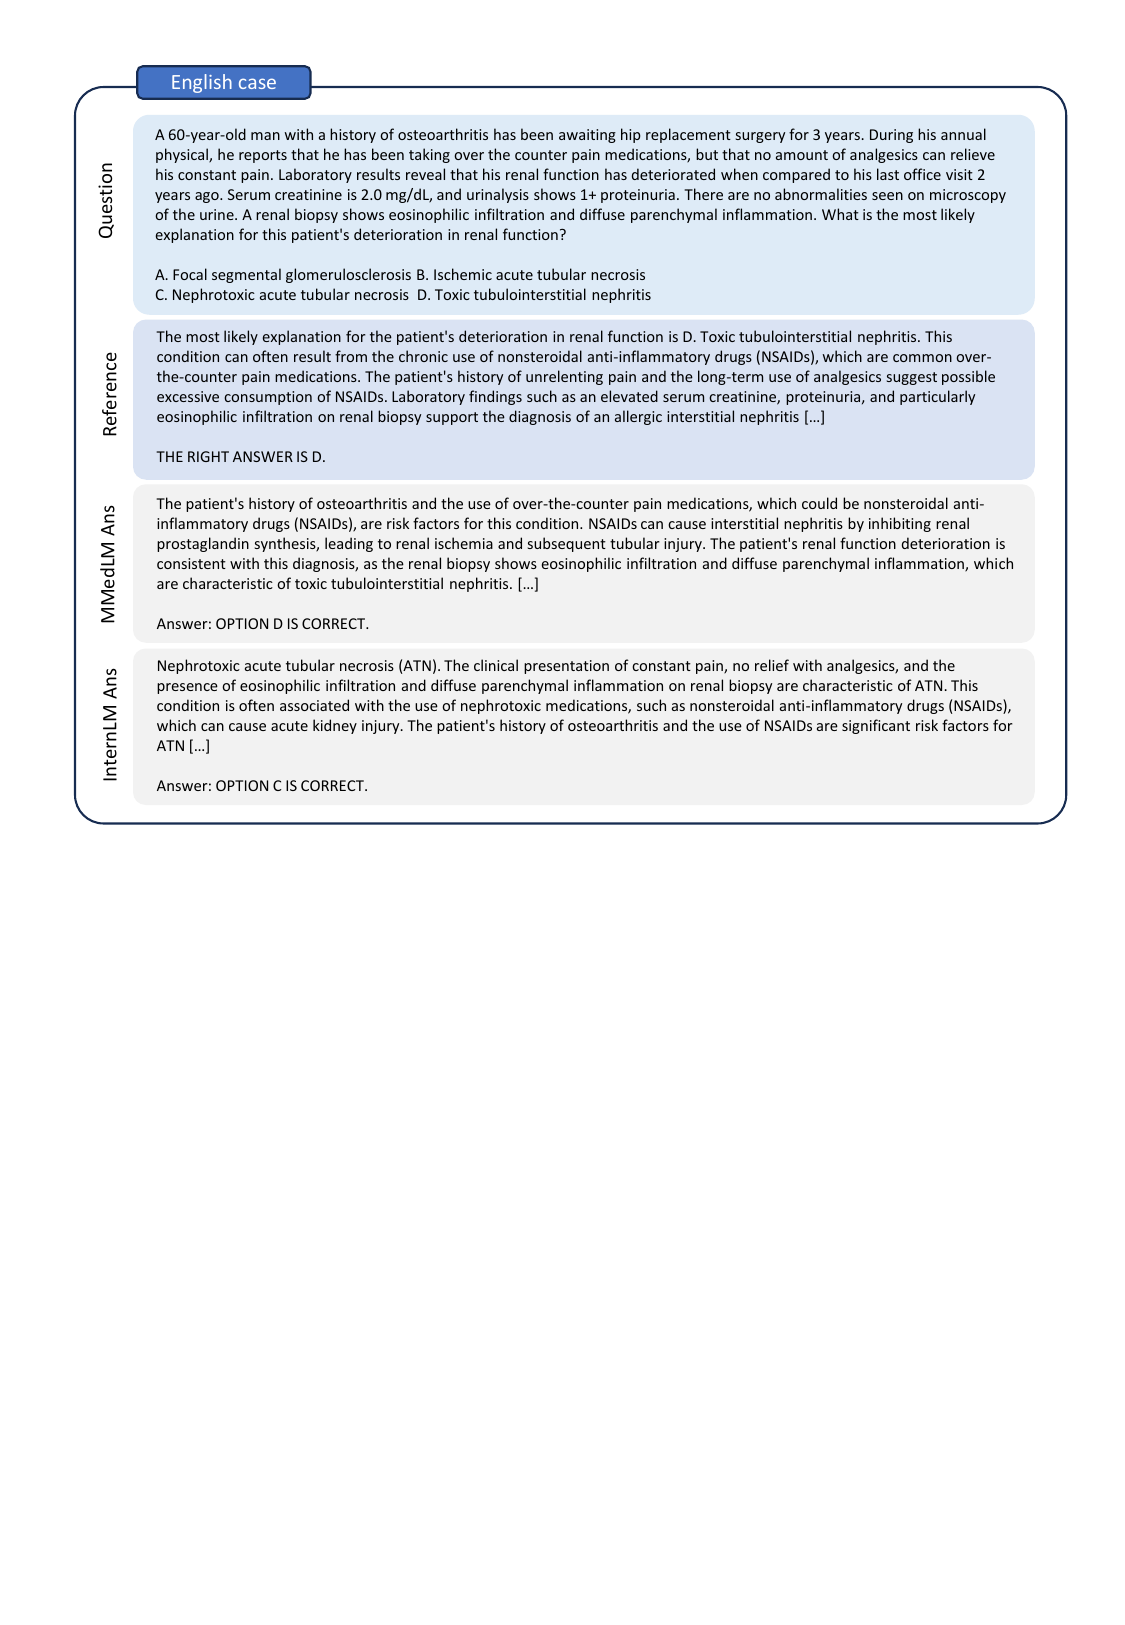}
    \vspace{-10pt}
    \caption{Case\ 1. An English case in MMedB.}
    \label{fig:case1}
\end{figure}

\begin{figure}[t]
    \centering
    \includegraphics[width=\textwidth]{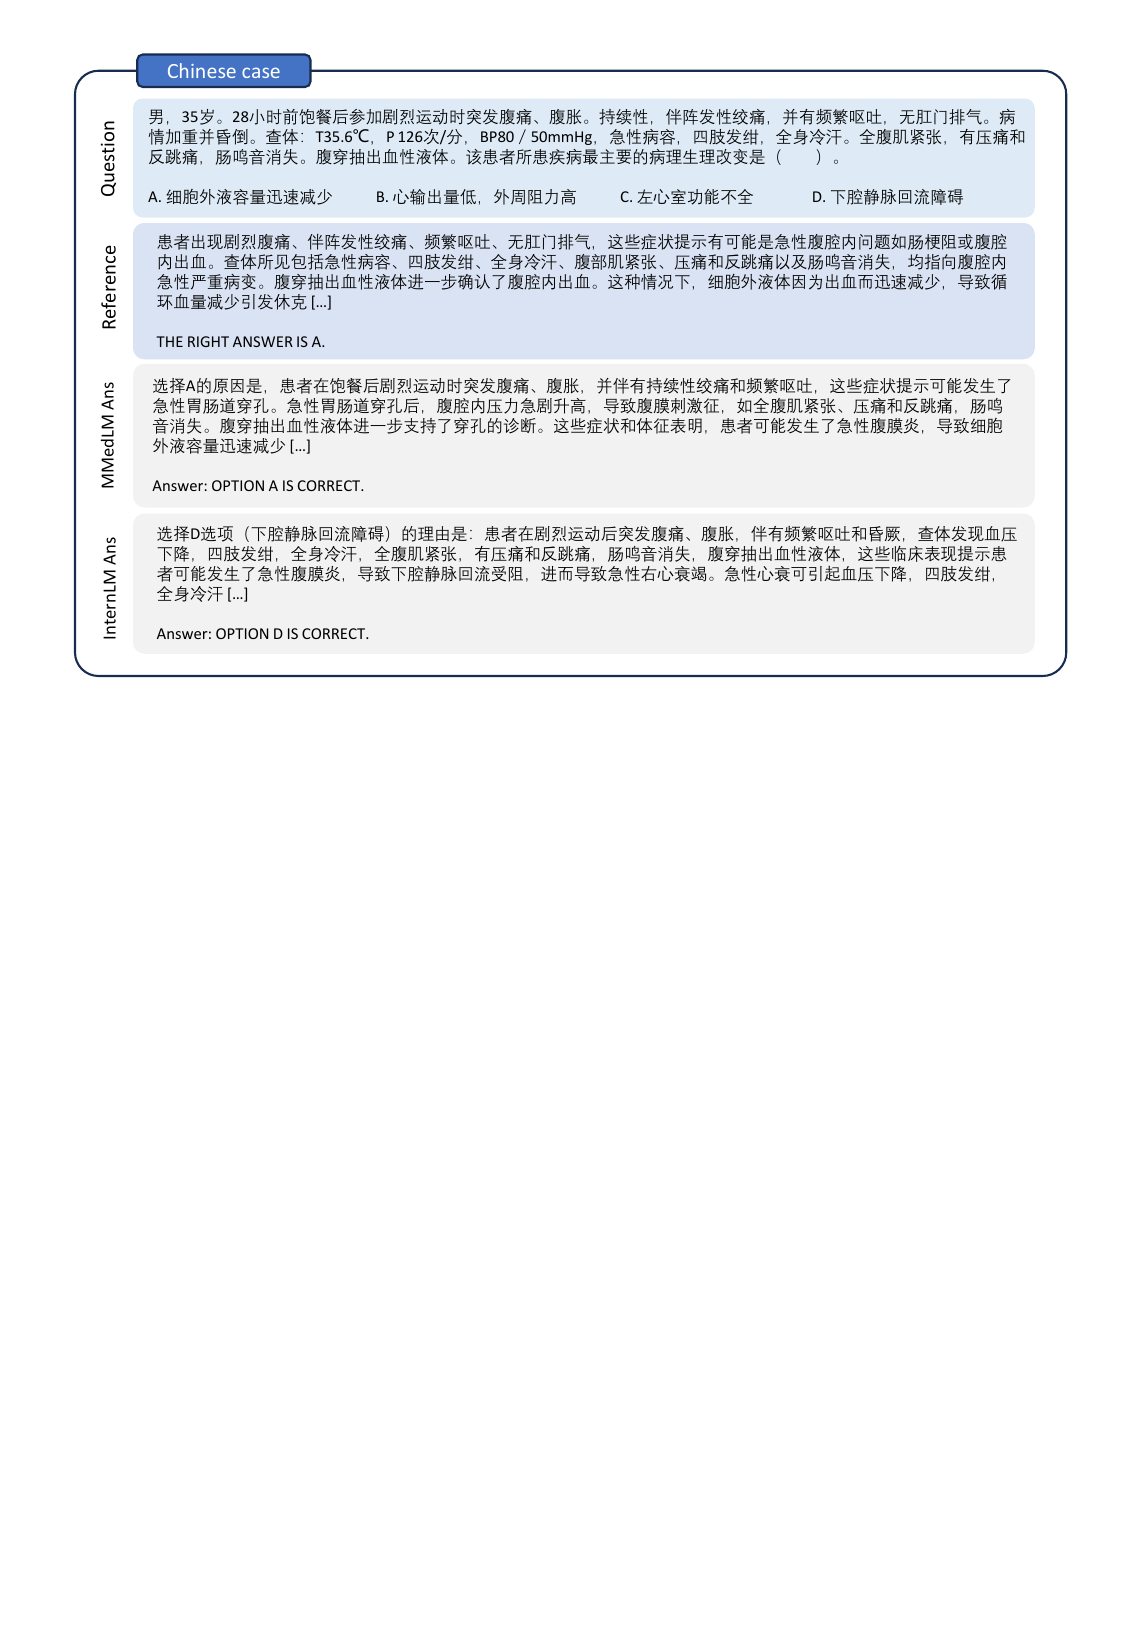}
    \vspace{-10pt}
    \caption{Case\ 2. An Chinese case in MMedB}
    \label{fig:case2}
\end{figure}

\begin{figure}[t]
    \centering
    \includegraphics[width=\textwidth]{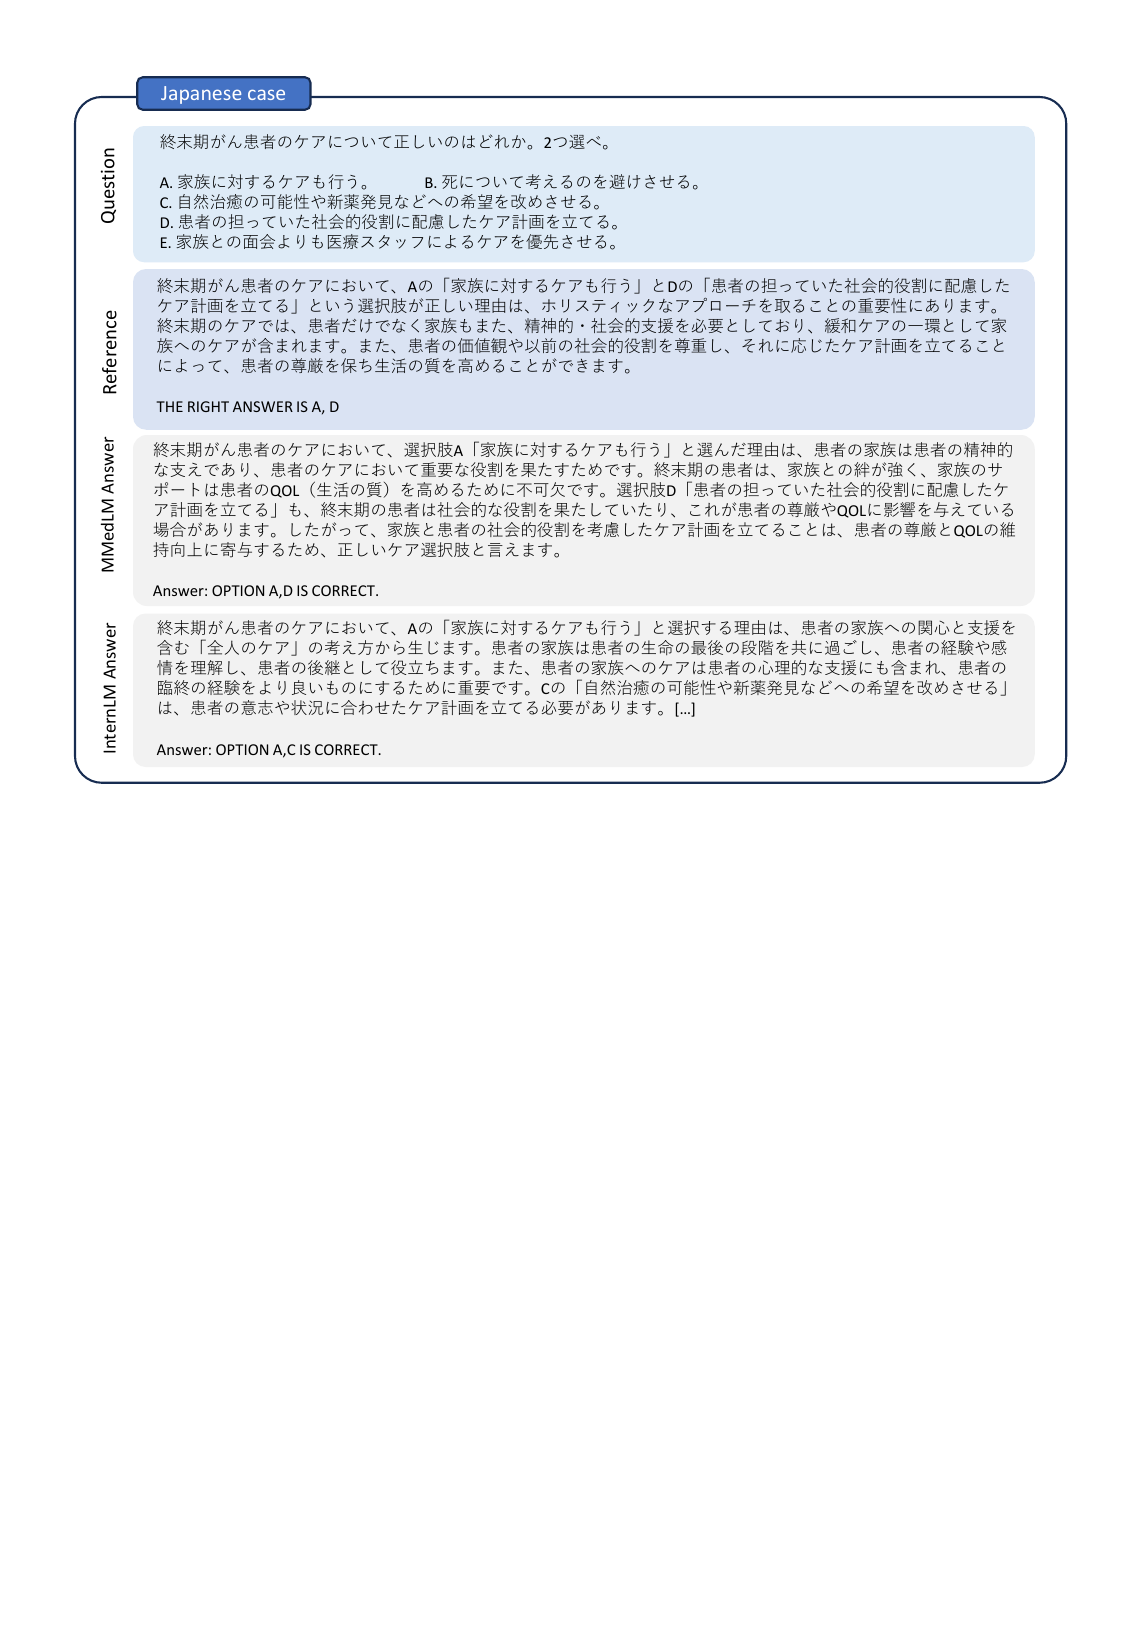}
    \vspace{-10pt}
    \caption{Case\ 3. An Japanese case in MMedB}
    \label{fig:case3}
\end{figure}

\begin{figure}[t]
    \centering
    \includegraphics[width=\textwidth]{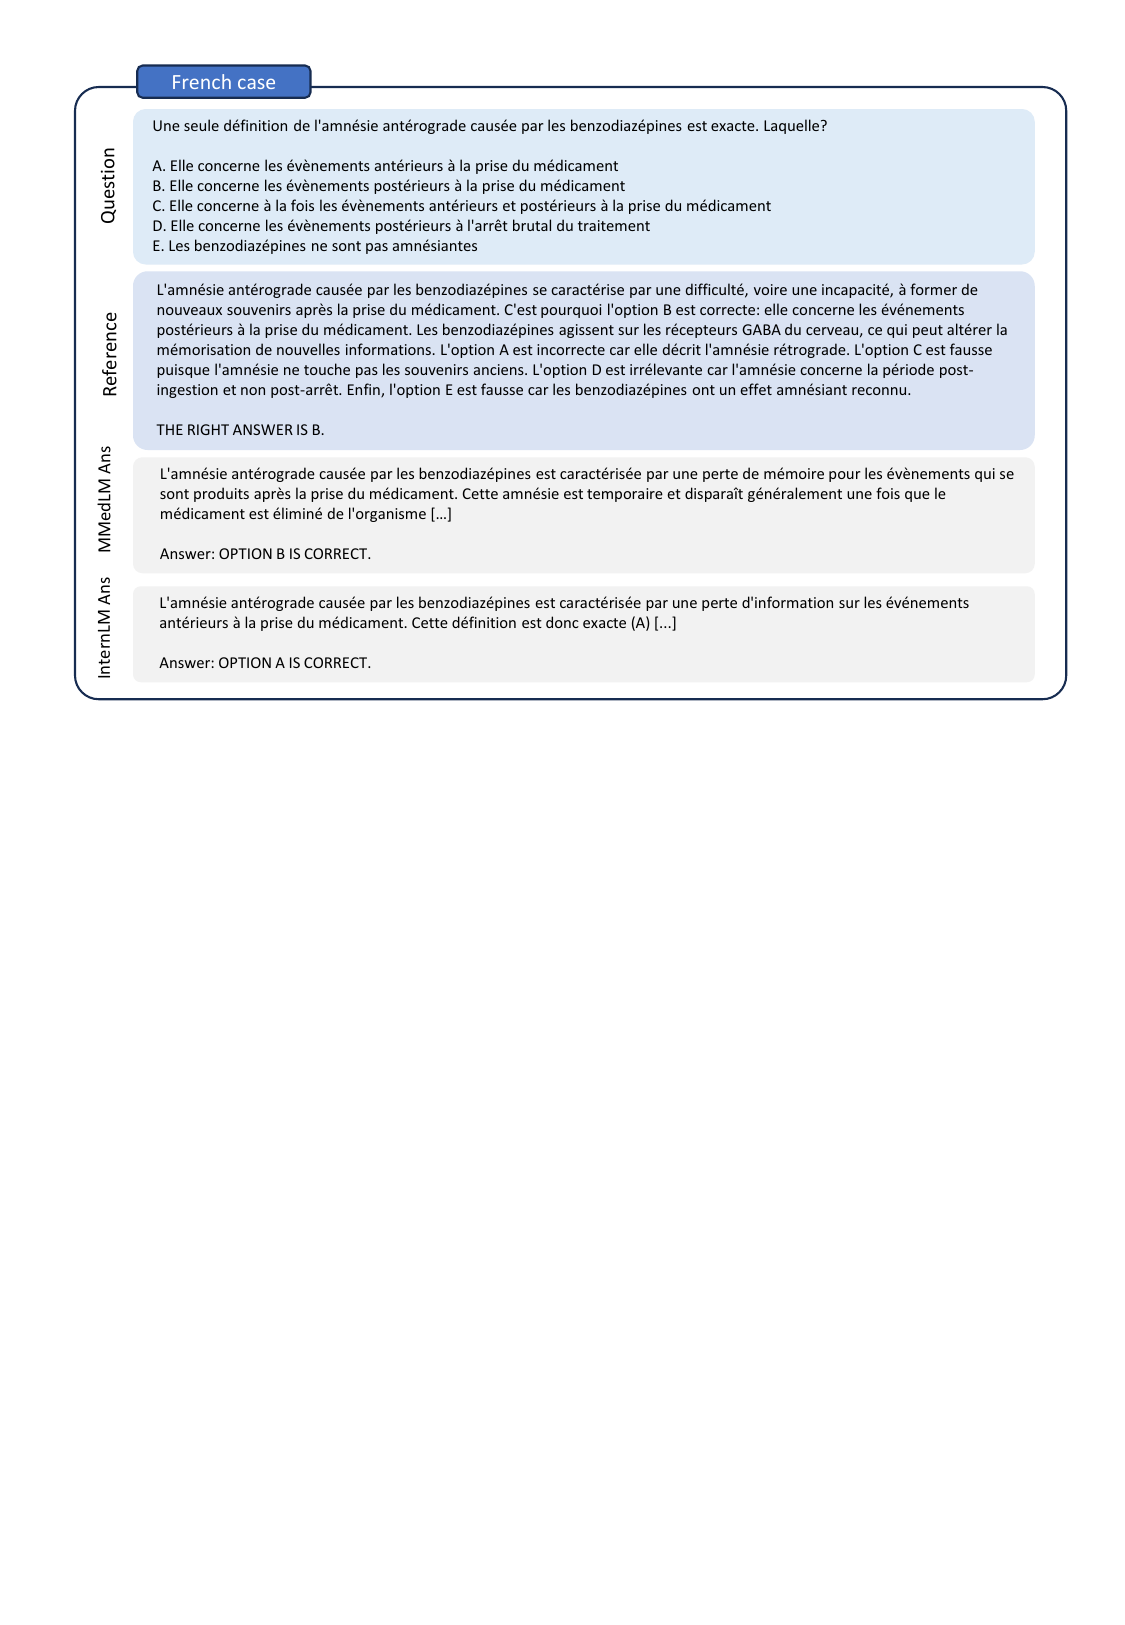}
    \vspace{-10pt}
    \caption{Case\ 4. An French case in MMedB}
    \label{fig:case4}
\end{figure}

\begin{figure}[t]
    \centering
    \includegraphics[width=\textwidth]{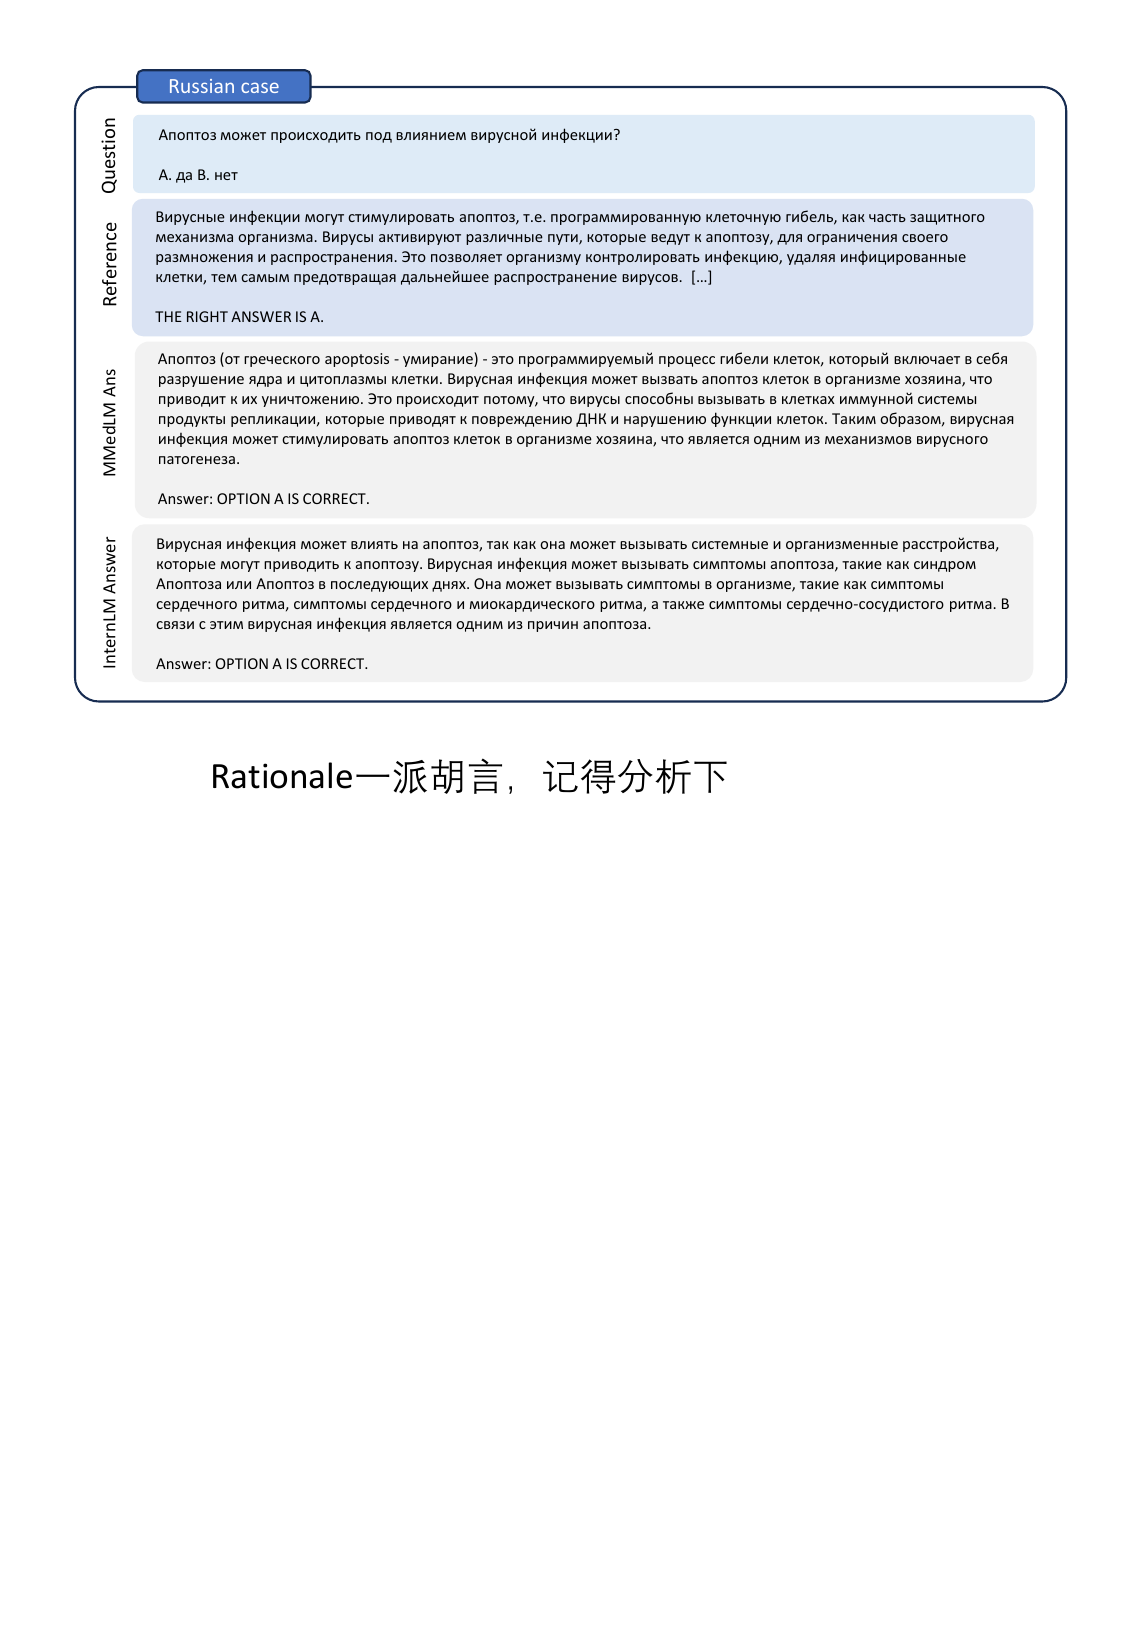}
    \vspace{-10pt}
    \caption{Case\ 5. An Russian case in MMedB}
    \label{fig:case5}
\end{figure}

\begin{figure}[t]
    \centering
    \includegraphics[width=\textwidth]{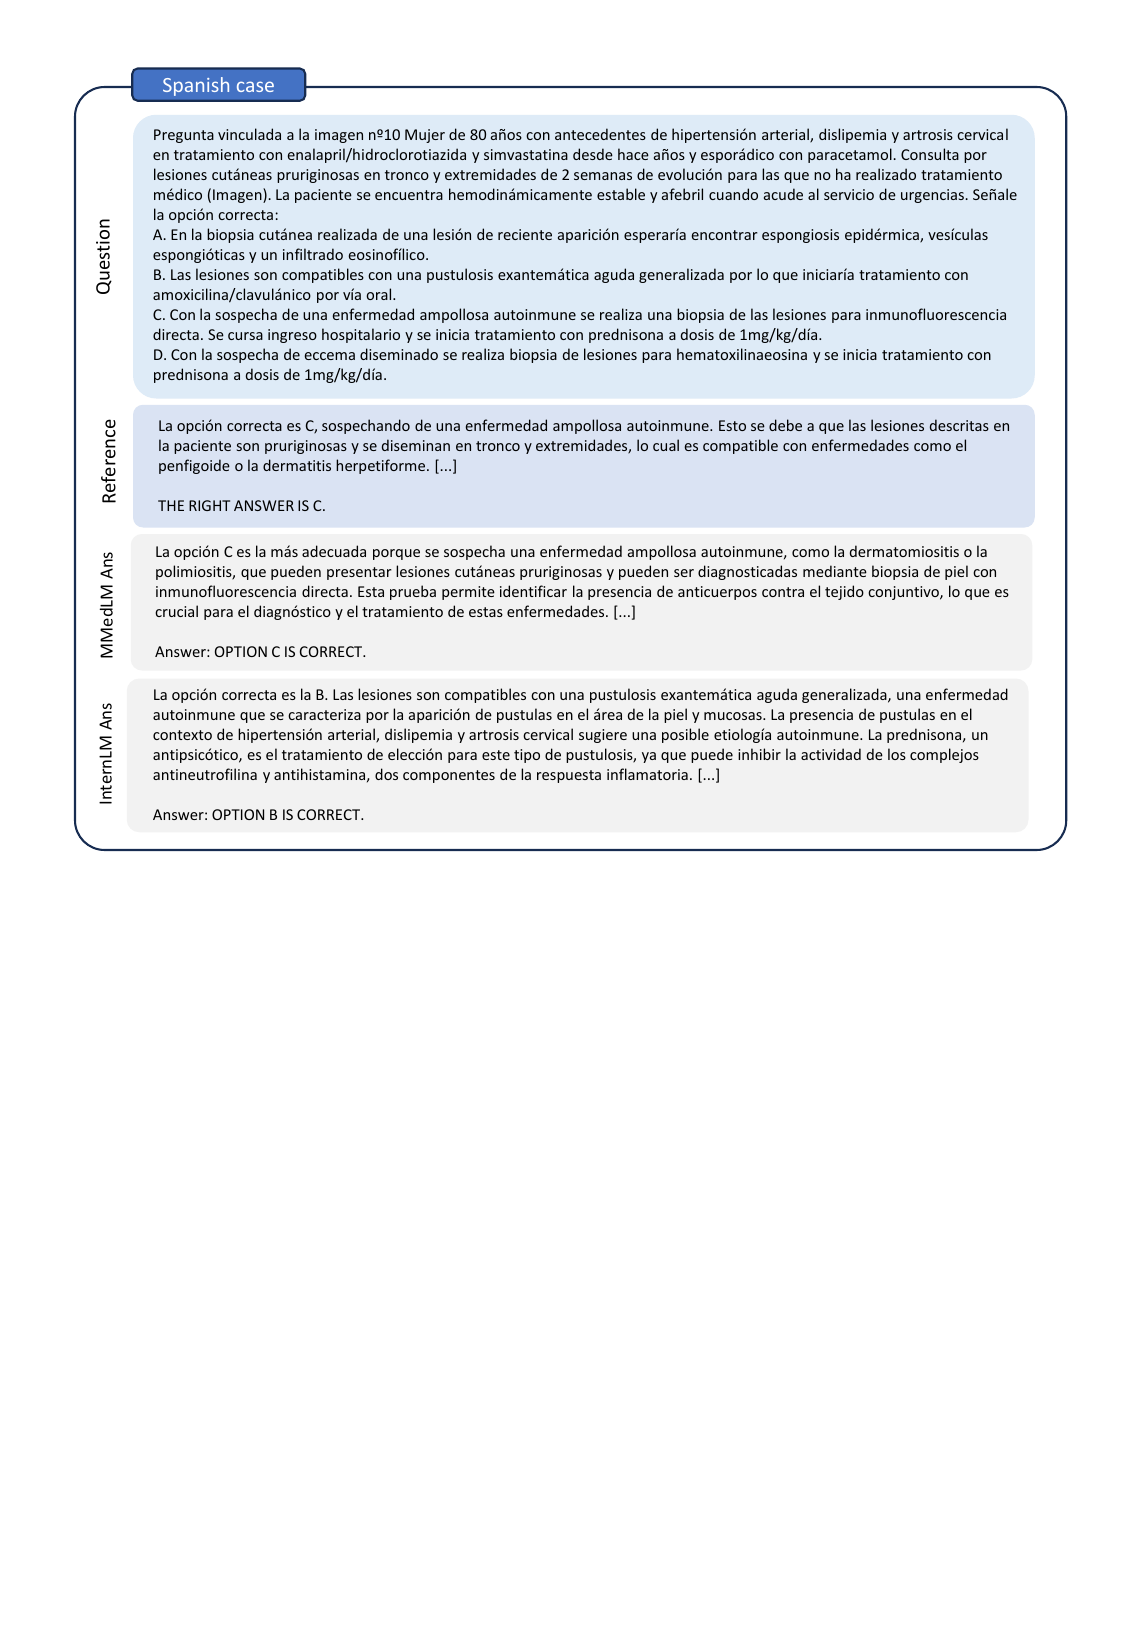}
    \vspace{-10pt}
    \caption{Case\ 6. An Spanish case in MMedB}
    \label{fig:case6}
\end{figure}
